# Supplementary material for: BuDDI: A Declarative Bloom Language for CALM Programming
Source: arXiv:2109.08192 source file (2021-09-20)
Supplement: Supplementary file 1 [file appendix.tex]

\section{Appendix}\label{sec:appendix}

\lstinputlisting[style=customc, label={lst:unicast}, caption={Reliable Unicast in Buddy}]{codes/reliable_unicast_monotone.py}

% \clearpage

% \lstinputlisting[style=customc, label={lst:kmerbuddy}, caption={KMER counting in Buddy}]{codes/kmer_b.py}

% \clearpage

% \subsection{K-mer Counting}
